# Supplementary material for: LayoutRectifier: An Optimization-based Post-processing for Graphic Design Layout Generation
Source: arXiv:2508.11177 source file (2025-08-23)
Supplement: Supplementary file 2 [file size_ablation_supp_fig.tex]

\begin{figure}
  \centering
  \includegraphics[width=\linewidth]{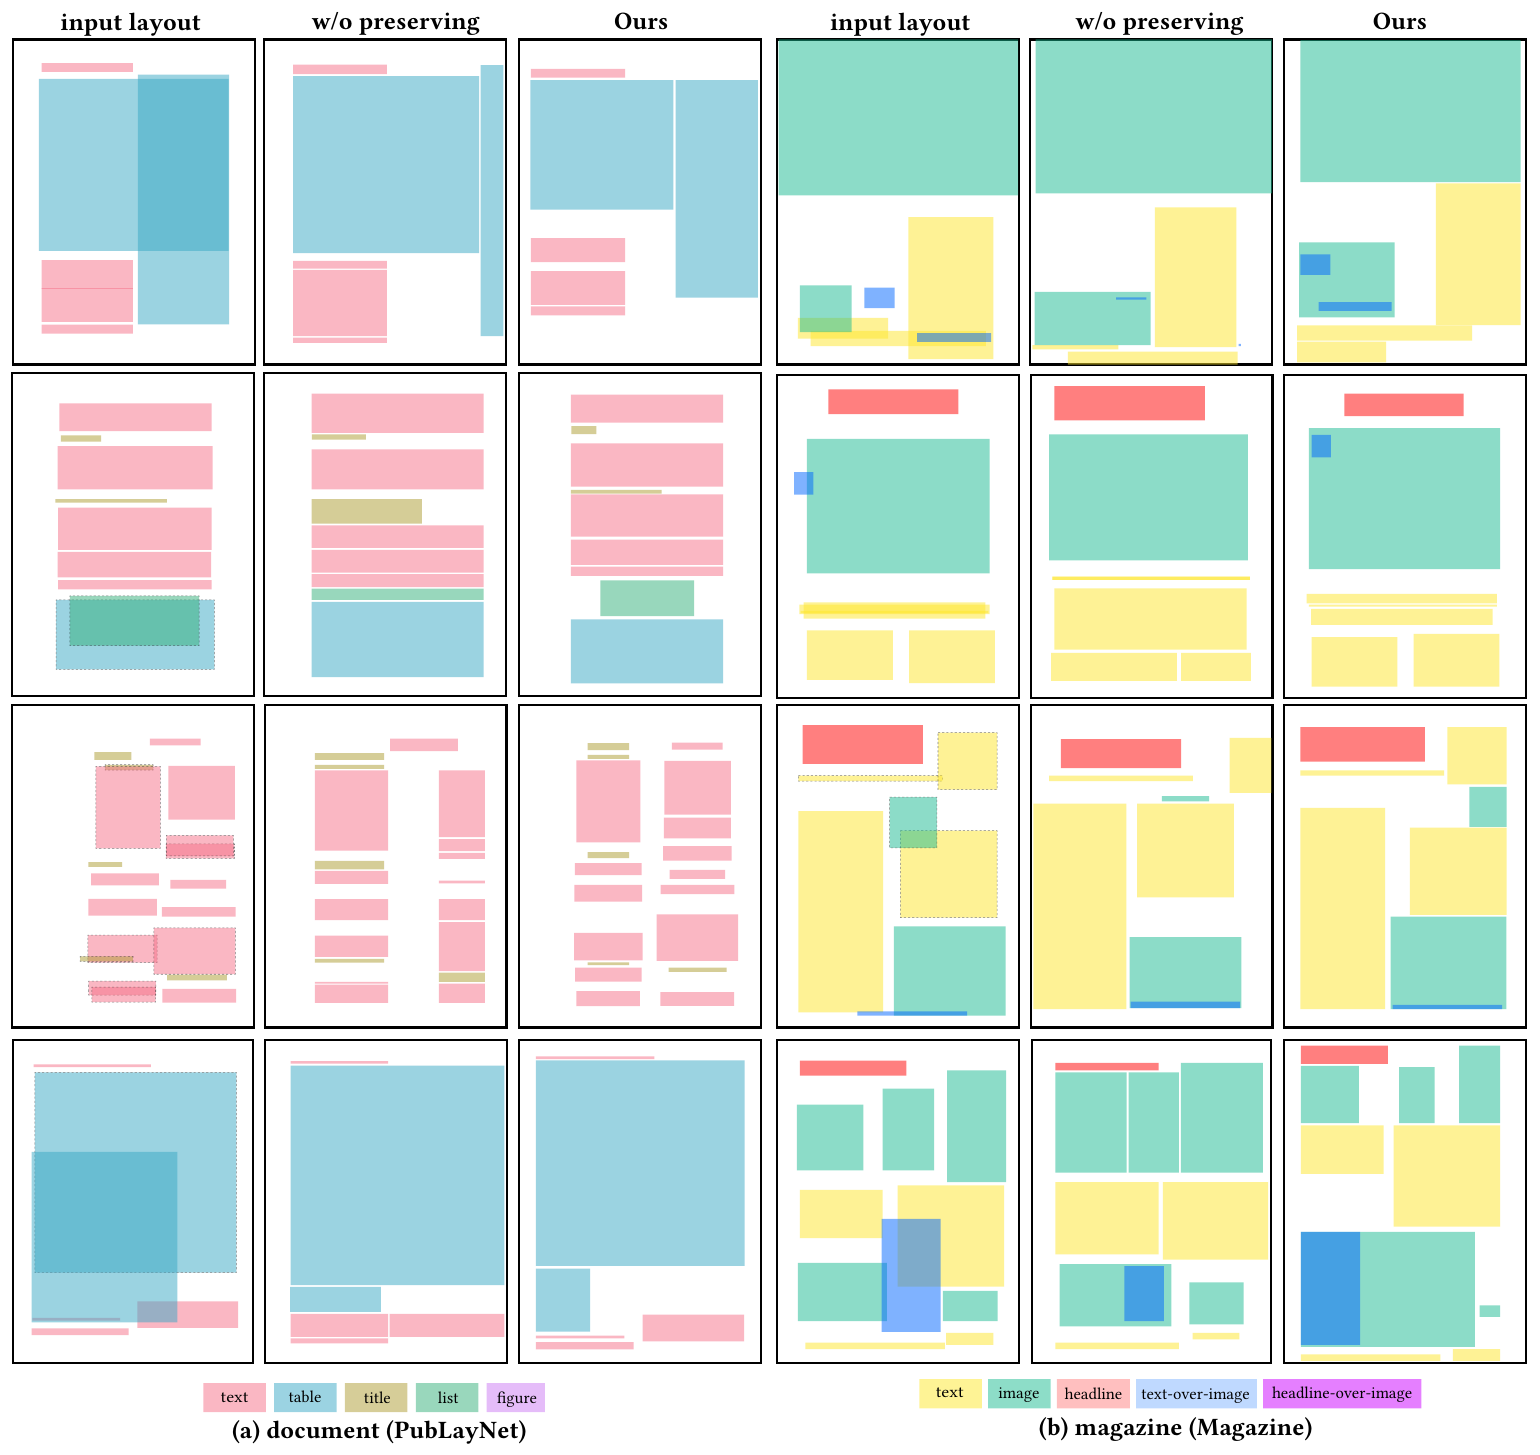}
  \caption{
% \todo{Check the figure carefully there is a wrong figure..}
  \textbf{Qualitative comparison of element preserving ablation study.} We compared the refined layouts generated with and without the size and aspect ratio preservation terms. 
    The size and aspect ratio of elements are better preserved in the layouts generated with the preservation terms. 
  }
  \label{fig:supp_size_ablation}
\end{figure}
